# Supplementary material for: Generation and symmetry control of high-dimensional quantum frequency states
Source: arXiv:1903.10385 ancillary file (2019-03-25)
Supplement: Supplementary file 1 [file Supplementary.pdf]

# Generation and symmetry control of high-dimensional quantum frequency states (Supplementary material)

G. Maltese,[1] M.I. Amanti*,[1] F. Appas,[1] G. Sinnl,[1] A. Lemaître,[2] P. Milman,[1] F.Baboux,[1] and S. Ducci[1]

[1] *Laboratoire Matériaux et Phénomènes Quantiques, Université Paris Diderot, CNRS-UMR 7162, Paris 75013, France*

[2] *Centre de Nanosciences et de Nanotechnologies, CNRS, Université Paris-Sud, Université Paris-Saclay, C2N-Marcoussis*

# JSA of a two-photon state at the output of a cavity.

As a complement to Figure 2 of the main text, we present in Supplementary Figure 1 the calculated JSA (real and imaginary part) of the quantum state generated by type II SPDC in presence of a Fabry Perot cavity of reflectivity 0.8, in the case of a pump laser centered at $\omega_R$ and of linewidth $\Delta\omega \gg \bar{\omega}$. Dashed lines show representative resonant and anti-resonant cuts of the JSA corresponding to results presented in Figure 2 (b)-(c).

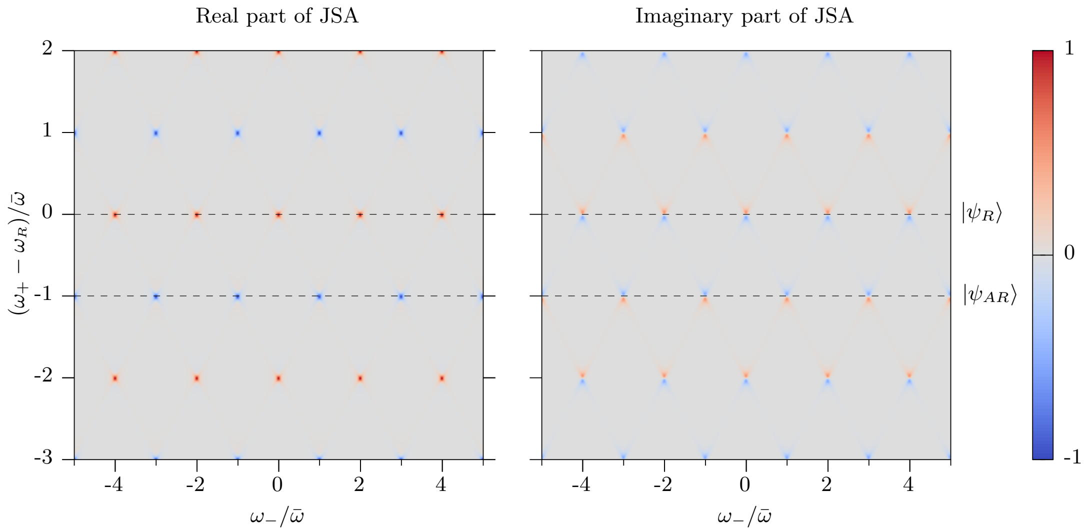


FIG. 1. Calculated JSA (real and imaginary part) of the quantum state generated by type II SPDC filtered by a Fabry Perot cavity of reflectivity 0.8, in the case of a pump laser centered at $\omega_R$ and of linewidth $\Delta\omega \gg \bar{\omega}$. Dashed lines show representative resonant and anti-resonant cuts of the JSA corresponding to results presented in Figure 2 (b)-(c) of the main text .

# Calculated JSA for different time delays.

In Figure 2 b-c/d-e of the main text we present the calculated JSA for temporal delay values of $\tau$=0 and $\tau = \frac{\pi}{\bar{\omega}}$. In Supplementary Figure 2 below we show the calculated JSA for additional delays $\tau = 0$, $\tau = \frac{\pi}{\bar{\omega}} + n\frac{2\pi}{\bar{\omega}}$, $\tau = \frac{2\pi}{\bar{\omega}} + n\frac{2\pi}{\bar{\omega}}$, $\tau = \frac{3\pi}{\bar{\omega}} + n\frac{2\pi}{\bar{\omega}}$, where $n$ is an integer number. We notice that results for $\tau = 0$, $\tau = \frac{\pi}{\bar{\omega}} + n\frac{2\pi}{\bar{\omega}}$ correspond to calculations in Figure 2 b-c/d-e.

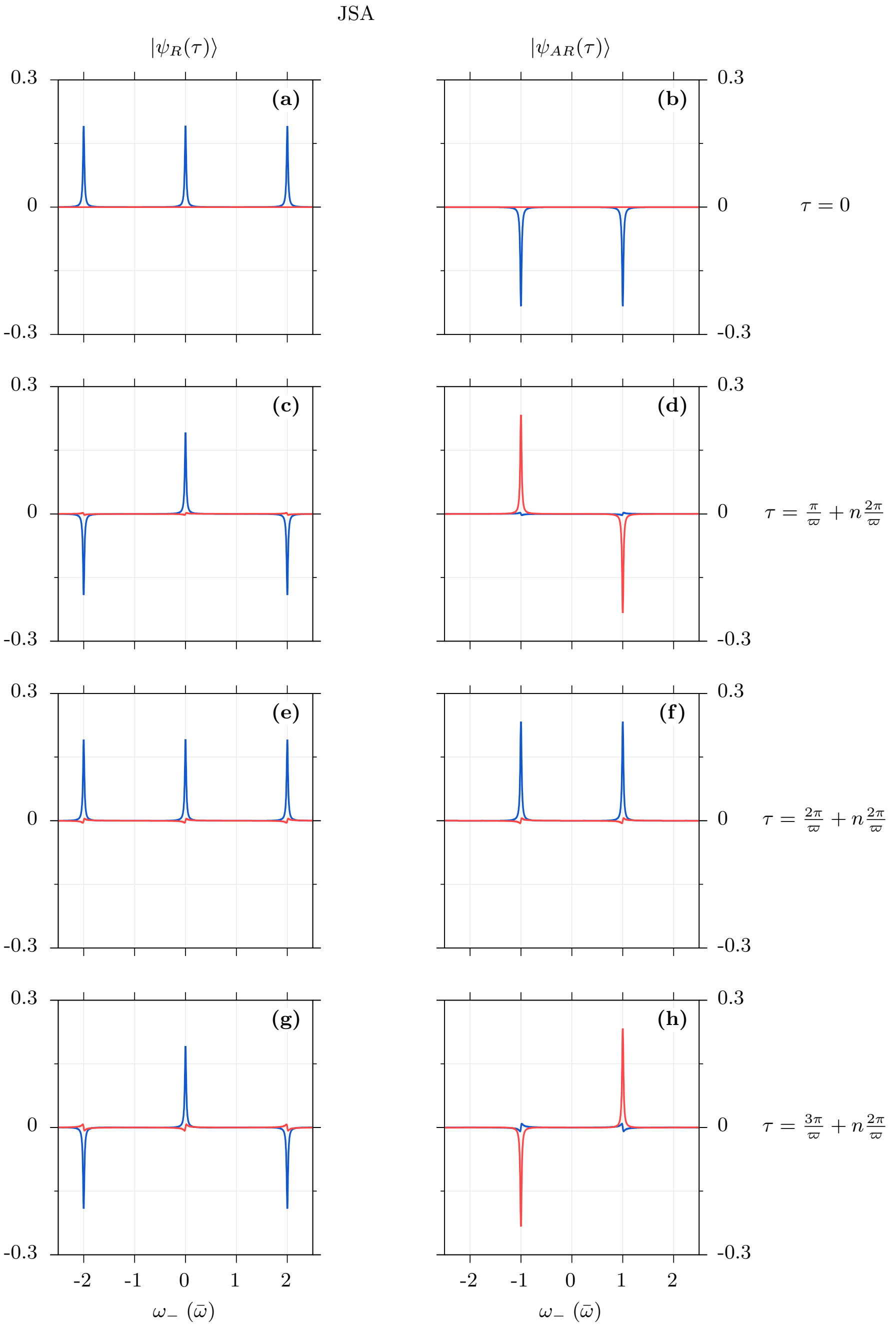


FIG. 2. Calculated JSA for the resonant (left) and anti-resonant state (right) for values of temporal delay of $\tau = 0$, $\tau = \frac{\pi}{\bar{\omega}} + n\frac{2\pi}{\bar{\omega}}$, $\tau = \frac{2\pi}{\bar{\omega}} + n\frac{2\pi}{\bar{\omega}}$, $\tau = \frac{3\pi}{\bar{\omega}} + n\frac{2\pi}{\bar{\omega}}$, where $n$ is an integer number.

# AlGaAs waveguide

In Supplementary Table I we present the epitaxial structure of the AlGaAs waveguide studied in the main text

| **Layer** | **Material** |
|---|---|
| Top Bragg (x6) | $Al_{0.25}Ga_{0.75}As$ |
| | $Al_{0.80}Ga_{0.20}As$ |
| Core (298nm) | $Al_{0.45}Ga_{0.55}As$ |
| Bottom Bragg (x6) | $Al_{0.80}Ga_{0.20}As$ |
| | $Al_{0.25}Ga_{0.75}As$ |
| Substrate | GaAs |

TABLE I. Nominal epitaxial structure of AlGaAs waveguide source.

# Calculated phase matching function and Hong Ou Mandel interferometry pattern for the AlGaAs waveguide.

In Supplementary Figure 3 we present the calculated phase matching function $C_{PM}$ for the AlGaAs chip presented in the main text. The effective refractive index of the modes propagating in the waveguide are obtained by EigenMode simulation via commercial available software.

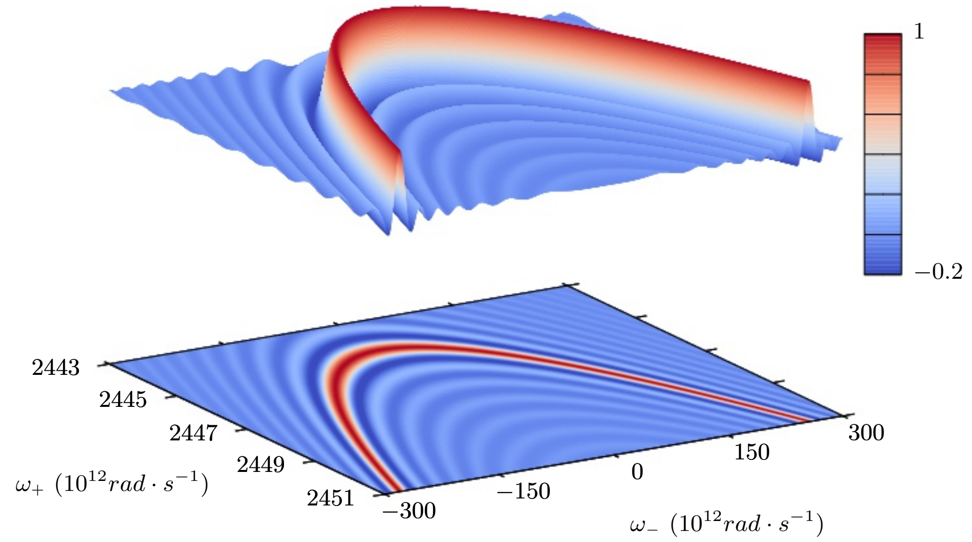


FIG. 3. Calculated phase matching function $C_{PM}$ for the AlGaAs chip presented in the main text, as function of $\omega_+$ and $\omega_-$

Starting from this phase-matching function, we present in Supplementary Figure 4 the corresponding calculated HOM interference pattern close to $\tau_{HOM} = 0$ in the case of a monochromatic pump, for $\omega_+$ values corresponding to the ones of Supplementary Figure 3.

By comparing this calculation with the experimental HOM interferometry measurement for $|\psi_R\rangle$, reported in Figure 4 of the main text, we estimate a two-photon bandwidth of $\Delta\omega_- = 137$ THz.

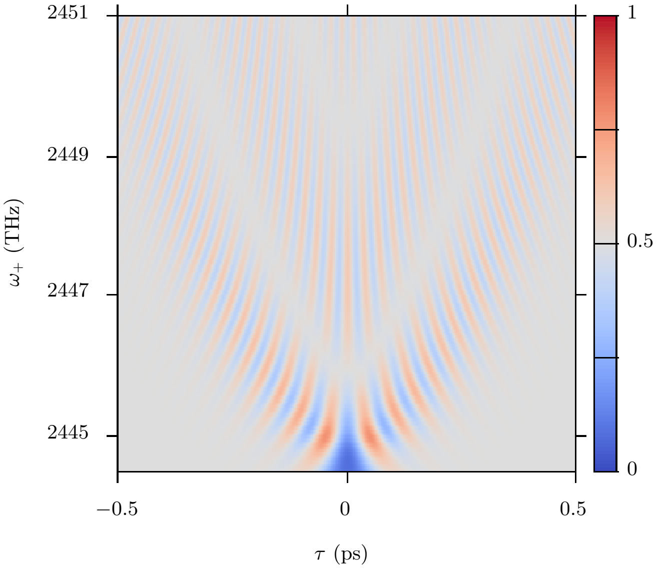


FIG. 4. Numerically simulated HOM interference pattern as a function of the pump frequency $\omega_+$ in the case of an AlGaAs waveguide, corresponding to the phase matching function in Figure 3.

# Impact of the cavity reflectivity on the HOM pattern.

In Supplementary Figure 5 we present the calculated HOM pattern as a function of the cavity reflectivity, in the ideal case of zero birefringence and zero chromatic dispersion for the AlGaAs waveguide. We investigate the case of resonant (left panel) and anti-resonant (right panel) quantum state. Peak and dip visibilities are strongly affected by cavity reflectivity.

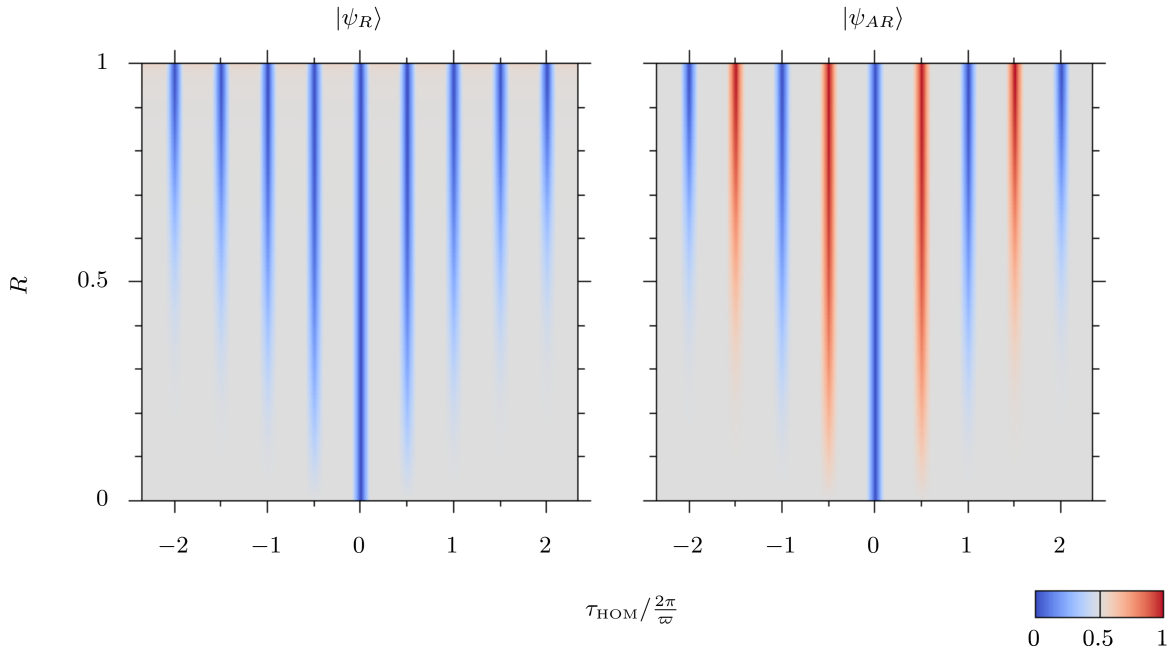


FIG. 5. Simulated results of HOM interferometry for a quantum state generated by type II SPDC in the case of zero birefringence and chromatic dispersion. Simulated coincidence probability as a function of the temporal delay between two photons in a pair ($\tau_{\text{HOM}}$) and of the reflectivity of the Fabry Perot cavity (on the y axis) in the case of resonant (left panel) and anti-resonant (right panel) states.
